# Supplementary material for: Synaptic Pruning: A Biological Inspiration for Deep Learning Regularization
Source: arXiv:2508.09330 source file (2025-10-05)
Supplement: Supplementary file 1 [file AppendixA.pdf]

# RNN Model Results

| Dataset | Model | Metric | Sequence Length | No Dropout | Dropout | MC Dropout | Synaptic Pruning |
|---|---|---|---|---|---|---|---|
| Bitcoin | RNN | mae | 1 | 0.3236 | 0.3152 | 0.3176 | 0.2900 |
| Bitcoin | RNN | runtime | 1 | 0.3705 | 0.3623 | 0.3737 | 0.3388 |
| Bitcoin | RNN | mae_95ci_low | 1 | 0.2491 | 0.2370 | 0.2330 | 0.2380 |
| Bitcoin | RNN | mae_95ci_high | 1 | 0.3981 | 0.3934 | 0.4023 | 0.3421 |
| Bitcoin | RNN | mae | 3 | 0.3113 | 0.2679 | 0.2969 | 0.2455 |
| Bitcoin | RNN | runtime | 3 | 0.3591 | 0.3167 | 0.3563 | 0.3047 |
| Bitcoin | RNN | mae_95ci_low | 3 | 0.2451 | 0.2043 | 0.2313 | 0.2117 |
| Bitcoin | RNN | mae_95ci_high | 3 | 0.3774 | 0.3314 | 0.3626 | 0.2794 |
| Bitcoin | RNN | mae | 7 | 0.3006 | 0.2564 | 0.2860 | 0.2681 |
| Bitcoin | RNN | rmse | 7 | 0.3466 | 0.3054 | 0.3434 | 0.3360 |
| Bitcoin | RNN | mae_95ci_low | 7 | 0.2118 | 0.1733 | 0.2039 | 0.1690 |
| Bitcoin | RNN | mae_95ci_high | 7 | 0.3894 | 0.3395 | 0.3680 | 0.3672 |
| Bitcoin | RNN | mae | 14 | 0.3180 | 0.2703 | 0.2864 | 0.2699 |
| Bitcoin | RNN | rmse | 14 | 0.3638 | 0.3175 | 0.3469 | 0.3189 |
| Bitcoin | RNN | mae_95ci_low | 14 | 0.2391 | 0.1928 | 0.2052 | 0.2166 |
| Bitcoin | RNN | mae_95ci_high | 14 | 0.3969 | 0.3478 | 0.3676 | 0.3232 |
| Bitcoin | RNN | mae | 30 | 0.3263 | 0.2954 | 0.3144 | 0.2395 |
| Bitcoin | RNN | rmse | 30 | 0.3695 | 0.3403 | 0.3698 | 0.2934 |
| Bitcoin | RNN | mae_95ci_low | 30 | 0.2699 | 0.2158 | 0.2269 | 0.1787 |
| Bitcoin | RNN | mae_95ci_high | 30 | 0.3826 | 0.3750 | 0.4018 | 0.3002 |
| Bitcoin | RNN | mae | 60 | 0.3976 | 0.3763 | 0.3701 | 0.2596 |
| Bitcoin | RNN | runtime | 60 | 0.4381 | 0.4175 | 0.4205 | 0.3117 |
| Bitcoin | RNN | mae_95ci_low | 60 | 0.2694 | 0.2536 | 0.2296 | 0.1040 |
| Bitcoin | RNN | mae_95ci_high | 60 | 0.5257 | 0.4990 | 0.5105 | 0.4152 |
| S&P500 | RNN | mae | 1 | 0.1062 | 0.1096 | 0.1668 | 0.1060 |
| S&P500 | RNN | rmse | 1 | 0.1449 | 0.1434 | 0.2182 | 0.1447 |
| S&P500 | RNN | mae_95ci_low | 1 | 0.0955 | 0.0947 | 0.1525 | 0.0952 |
| S&P500 | RNN | mae_95ci_high | 1 | 0.1170 | 0.1245 | 0.1811 | 0.1168 |
| S&P500 | RNN | mae | 3 | 0.1204 | 0.1285 | 0.1571 | 0.1205 |
| S&P500 | RNN | rmse | 3 | 0.1595 | 0.1655 | 0.2061 | 0.1596 |
| S&P500 | RNN | mae_95ci_low | 3 | 0.0941 | 0.0995 | 0.1364 | 0.0940 |
| S&P500 | RNN | mae_95ci_high | 3 | 0.1468 | 0.1576 | 0.1778 | 0.1470 |

| | | | | | | | |
|---|---|---|---|---|---|---|---|
| S&P500 | RNN | mae | 7 | 0.0792 | 0.0951 | 0.1437 | 0.0792 |
| S&P500 | RNN | rmse | 7 | 0.1095 | 0.1254 | 0.1880 | 0.1095 |
| S&P500 | RNN | mae_95ci_low | 7 | 0.0631 | 0.0766 | 0.1297 | 0.0628 |
| S&P500 | RNN | mae_95ci_high | 7 | 0.0954 | 0.1136 | 0.1576 | 0.0955 |
| S&P500 | RNN | mae | 14 | 0.0845 | 0.1082 | 0.1500 | 0.0845 |
| S&P500 | RNN | rmse | 14 | 0.1147 | 0.1372 | 0.1953 | 0.1148 |
| S&P500 | RNN | mae_95ci_low | 14 | 0.0636 | 0.0646 | 0.1300 | 0.0638 |
| S&P500 | RNN | mae_95ci_high | 14 | 0.1053 | 0.1517 | 0.1701 | 0.1053 |
| S&P500 | RNN | mae | 30 | 0.0879 | 0.1104 | 0.1478 | 0.0878 |
| S&P500 | RNN | rmse | 30 | 0.1184 | 0.1410 | 0.1928 | 0.1184 |
| S&P500 | RNN | mae_95ci_low | 30 | 0.0679 | 0.0835 | 0.1290 | 0.0679 |
| S&P500 | RNN | mae_95ci_high | 30 | 0.1079 | 0.1373 | 0.1666 | 0.1078 |
| S&P500 | RNN | mae | 60 | 0.0883 | 0.1113 | 0.1558 | 0.0884 |
| S&P500 | RNN | rmse | 60 | 0.1182 | 0.1414 | 0.2024 | 0.1184 |
| S&P500 | RNN | mae_95ci_low | 60 | 0.0669 | 0.0815 | 0.1310 | 0.0670 |
| S&P500 | RNN | mae_95ci_high | 60 | 0.1097 | 0.1412 | 0.1807 | 0.1098 |
| Air Quality | RNN | mae | 1 | 0.8347 | 0.6915 | 0.7412 | 0.6881 |
| Air Quality | RNN | rmse | 1 | 1.0609 | 0.9188 | 0.9691 | 0.9360 |
| Air Quality | RNN | mae_95ci_low | 1 | 0.8123 | 0.6746 | 0.7323 | 0.6723 |
| Air Quality | RNN | mae_95ci_high | 1 | 0.8570 | 0.7084 | 0.7501 | 0.7039 |
| Air Quality | RNN | mae | 3 | 0.8404 | 0.7604 | 0.7875 | 0.7087 |
| Air Quality | RNN | rmse | 3 | 1.0879 | 0.9909 | 1.0193 | 0.9513 |
| Air Quality | RNN | mae_95ci_low | 3 | 0.7925 | 0.7190 | 0.7583 | 0.6863 |
| Air Quality | RNN | mae_95ci_high | 3 | 0.8883 | 0.8018 | 0.8168 | 0.7311 |
| Air Quality | RNN | mae | 7 | 0.8287 | 0.7498 | 0.8190 | 0.7337 |
| Air Quality | RNN | rmse | 7 | 1.0739 | 0.9904 | 1.0595 | 0.9621 |
| Air Quality | RNN | mae_95ci_low | 7 | 0.7820 | 0.7334 | 0.7832 | 0.6999 |
| Air Quality | RNN | mae_95ci_high | 7 | 0.8754 | 0.7663 | 0.8548 | 0.7674 |
| Air Quality | RNN | mae | 14 | 0.8128 | 0.7715 | 0.8137 | 0.7440 |
| Air Quality | RNN | rmse | 14 | 1.0479 | 1.0050 | 1.0496 | 0.9772 |
| Air Quality | RNN | mae_95ci_low | 14 | 0.7637 | 0.7429 | 0.7844 | 0.6950 |
| Air Quality | RNN | mae_95ci_high | 14 | 0.8619 | 0.8000 | 0.8429 | 0.7930 |
| Air Quality | RNN | mae | 30 | 0.8625 | 0.7968 | 0.8138 | 0.7655 |
| Air Quality | RNN | rmse | 30 | 1.1118 | 1.0278 | 1.0515 | 0.9994 |
| Air Quality | RNN | mae_95ci_low | 30 | 0.8098 | 0.7505 | 0.7740 | 0.6988 |
| Air Quality | RNN | mae_95ci_high | 30 | 0.9152 | 0.8430 | 0.8537 | 0.8321 |

| | | | | | | | |
|---|---|---|---|---|---|---|---|
| Air Quality | RNN | mae | 60 | 0.7996 | 0.7713 | 0.8200 | 0.7190 |
| Air Quality | RNN | rmse | 60 | 1.0317 | 1.0042 | 1.0541 | 0.9550 |
| Air Quality | RNN | mae_95ci_low | 60 | 0.7536 | 0.7331 | 0.7921 | 0.6860 |
| Air Quality | RNN | mae_95ci_high | 60 | 0.8456 | 0.8095 | 0.8478 | 0.7520 |
| Electricity | RNN | mae | 1 | 0.0817 | 0.0806 | 0.1043 | 0.0814 |
| Electricity | RNN | rmse | 1 | 0.1980 | 0.1998 | 0.2125 | 0.1982 |
| Electricity | RNN | mae_95ci_low | 1 | 0.0793 | 0.0767 | 0.1019 | 0.0783 |
| Electricity | RNN | mae_95ci_high | 1 | 0.0840 | 0.0845 | 0.1067 | 0.0845 |
| Electricity | RNN | mae | 3 | 0.0928 | 0.0886 | 0.1116 | 0.0899 |
| Electricity | RNN | rmse | 3 | 0.2018 | 0.2022 | 0.2172 | 0.2005 |
| Electricity | RNN | mae_95ci_low | 3 | 0.0864 | 0.0817 | 0.1075 | 0.0823 |
| Electricity | RNN | mae_95ci_high | 3 | 0.0992 | 0.0954 | 0.1158 | 0.0974 |
| Electricity | RNN | mae | 7 | 0.0922 | 0.0922 | 0.1143 | 0.0900 |
| Electricity | RNN | rmse | 7 | 0.2019 | 0.2025 | 0.2194 | 0.2000 |
| Electricity | RNN | mae_95ci_low | 7 | 0.0861 | 0.0786 | 0.1103 | 0.0840 |
| Electricity | RNN | mae_95ci_high | 7 | 0.0982 | 0.1058 | 0.1183 | 0.0960 |
| Electricity | RNN | mae | 14 | 0.0932 | 0.0887 | 0.1117 | 0.0845 |
| Electricity | RNN | rmse | 14 | 0.1995 | 0.2026 | 0.2176 | 0.1970 |
| Electricity | RNN | mae_95ci_low | 14 | 0.0862 | 0.0833 | 0.1088 | 0.0792 |
| Electricity | RNN | mae_95ci_high | 14 | 0.1002 | 0.0941 | 0.1147 | 0.0898 |
| Electricity | RNN | mae | 30 | 0.0915 | 0.0838 | 0.1122 | 0.0830 |
| Electricity | RNN | rmse | 30 | 0.1966 | 0.1986 | 0.2184 | 0.1934 |
| Electricity | RNN | mae_95ci_low | 30 | 0.0857 | 0.0795 | 0.1083 | 0.0792 |
| Electricity | RNN | mae_95ci_high | 30 | 0.0972 | 0.0881 | 0.1161 | 0.0868 |
| Electricity | RNN | mae | 60 | 0.0895 | 0.0919 | 0.1109 | 0.0839 |
| Electricity | RNN | rmse | 60 | 0.1958 | 0.2005 | 0.2159 | 0.1940 |
| Electricity | RNN | mae_95ci_low | 60 | 0.0856 | 0.0843 | 0.1066 | 0.0806 |
| Electricity | RNN | mae_95ci_high | 60 | 0.0933 | 0.0995 | 0.1153 | 0.0872 |

# LSTM Model Results

| Dataset | Model | Metric | Sequence Length | No Dropout | Dropout | MC Dropout | Synaptic Pruning |
|---|---|---|---|---|---|---|---|
| Bitcoin | LSTM | mae | 1 | 0.2447 | 0.2444 | 0.2551 | 0.2359 |
| Bitcoin | LSTM | runtime | 1 | 0.1190 | 0.1079 | 0.1176 | 1.8706 |
| Bitcoin | LSTM | mae_95ci_low | 1 | 0.2343 | 0.2346 | 0.2438 | 0.2249 |
| Bitcoin | LSTM | mae_95ci_high | 1 | 0.2551 | 0.2542 | 0.2664 | 0.2468 |
| Bitcoin | LSTM | mae | 3 | 0.4187 | 0.4072 | 0.4104 | 0.3513 |
| Bitcoin | LSTM | runtime | 3 | 0.0674 | 0.0697 | 0.0725 | 1.0815 |
| Bitcoin | LSTM | mae_95ci_low | 3 | 0.3914 | 0.3813 | 0.3832 | 0.3339 |
| Bitcoin | LSTM | mae_95ci_high | 3 | 0.4460 | 0.4330 | 0.4376 | 0.3686 |
| Bitcoin | LSTM | mae | 7 | 0.4992 | 0.4756 | 0.4832 | 0.4522 |
| Bitcoin | LSTM | runtime | 7 | 0.0713 | 0.0720 | 0.0808 | 0.8494 |
| Bitcoin | LSTM | mae_95ci_low | 7 | 0.4273 | 0.4074 | 0.4082 | 0.4250 |
| Bitcoin | LSTM | mae_95ci_high | 7 | 0.5711 | 0.5437 | 0.5582 | 0.4794 |
| Bitcoin | LSTM | mae | 14 | 0.5430 | 0.5197 | 0.4818 | 0.4914 |
| Bitcoin | LSTM | runtime | 14 | 0.0704 | 0.0717 | 0.1031 | 0.9094 |
| Bitcoin | LSTM | mae_95ci_low | 14 | 0.4722 | 0.4473 | 0.3992 | 0.4431 |
| Bitcoin | LSTM | mae_95ci_high | 14 | 0.6138 | 0.5922 | 0.5645 | 0.5398 |
| Bitcoin | LSTM | mae | 30 | 0.5586 | 0.5430 | 0.5425 | 0.5265 |
| Bitcoin | LSTM | runtime | 30 | 0.0666 | 0.0721 | 0.0772 | 0.7618 |
| Bitcoin | LSTM | mae_95ci_low | 30 | 0.4872 | 0.4715 | 0.4639 | 0.4842 |
| Bitcoin | LSTM | mae_95ci_high | 30 | 0.6301 | 0.6146 | 0.6210 | 0.5688 |
| Bitcoin | LSTM | mae | 60 | 0.6182 | 0.6096 | 0.6042 | 0.4701 |
| Bitcoin | LSTM | rmse | 60 | 0.6526 | 0.6443 | 0.6499 | 0.5116 |
| Bitcoin | LSTM | mae_95ci_low | 60 | 0.5826 | 0.5792 | 0.5737 | 0.4454 |
| Bitcoin | LSTM | mae_95ci_high | 60 | 0.6537 | 0.6400 | 0.6347 | 0.4949 |
| S&P500 | LSTM | mae | 1 | 0.6263 | 0.6384 | 0.6374 | 0.6260 |
| S&P500 | LSTM | runtime | 1 | 0.5891 | 0.6019 | 0.6050 | 1.3054 |
| S&P500 | LSTM | mae_95ci_low | 1 | 0.5950 | 0.6119 | 0.6122 | 0.5945 |
| S&P500 | LSTM | mae_95ci_high | 1 | 0.6576 | 0.6649 | 0.6625 | 0.6575 |
| S&P500 | LSTM | mae | 3 | 0.5063 | 0.5251 | 0.5272 | 0.5061 |
| S&P500 | LSTM | runtime | 3 | 0.6354 | 0.6515 | 0.6580 | 1.3512 |
| S&P500 | LSTM | mae_95ci_low | 3 | 0.4747 | 0.5022 | 0.5017 | 0.4737 |
| S&P500 | LSTM | mae_95ci_high | 3 | 0.5379 | 0.5480 | 0.5526 | 0.5386 |

| | | | | | | | |
|---|---|---|---|---|---|---|---|
| S&P500 | LSTM | mae | 7 | 0.4444 | 0.4815 | 0.4966 | 0.4445 |
| S&P500 | LSTM | runtime | 7 | 0.7500 | 0.7645 | 0.7568 | 1.4485 |
| S&P500 | LSTM | mae_95ci_low | 7 | 0.4071 | 0.4512 | 0.4571 | 0.4064 |
| S&P500 | LSTM | mae_95ci_high | 7 | 0.4818 | 0.5117 | 0.5360 | 0.4826 |
| S&P500 | LSTM | mae | 14 | 0.4249 | 0.4845 | 0.4943 | 0.4242 |
| S&P500 | LSTM | runtime | 14 | 0.8765 | 0.8859 | 0.9057 | 1.5774 |
| S&P500 | LSTM | mae_95ci_low | 14 | 0.3822 | 0.4492 | 0.4682 | 0.3806 |
| S&P500 | LSTM | mae_95ci_high | 14 | 0.4675 | 0.5199 | 0.5204 | 0.4678 |
| S&P500 | LSTM | mae | 30 | 0.3963 | 0.4631 | 0.4675 | 0.3960 |
| S&P500 | LSTM | runtime | 30 | 1.1833 | 1.1958 | 1.1878 | 1.8796 |
| S&P500 | LSTM | mae_95ci_low | 30 | 0.3557 | 0.4289 | 0.4268 | 0.3553 |
| S&P500 | LSTM | mae_95ci_high | 30 | 0.4368 | 0.4972 | 0.5081 | 0.4367 |
| S&P500 | LSTM | mae | 60 | 0.3794 | 0.4434 | 0.4381 | 0.3790 |
| S&P500 | LSTM | runtime | 60 | 1.7871 | 1.8529 | 1.8439 | 2.4188 |
| S&P500 | LSTM | mae_95ci_low | 60 | 0.3411 | 0.4067 | 0.4049 | 0.3398 |
| S&P500 | LSTM | mae_95ci_high | 60 | 0.4177 | 0.4801 | 0.4713 | 0.4181 |
| Air Quality | LSTM | mae | 1 | 0.8058 | 0.7439 | 0.7832 | 0.7418 |
| Air Quality | LSTM | rmse | 1 | 1.0676 | 0.9933 | 1.0397 | 0.9920 |
| Air Quality | LSTM | mae_95ci_low | 1 | 0.7660 | 0.7327 | 0.7550 | 0.7214 |
| Air Quality | LSTM | mae_95ci_high | 1 | 0.8455 | 0.7551 | 0.8114 | 0.7621 |
| Air Quality | LSTM | mae | 3 | 0.8256 | 0.7639 | 0.8111 | 0.7861 |
| Air Quality | LSTM | rmse | 3 | 1.1091 | 1.0337 | 1.0868 | 1.0505 |
| Air Quality | LSTM | mae_95ci_low | 3 | 0.7956 | 0.7341 | 0.7922 | 0.7521 |
| Air Quality | LSTM | mae_95ci_high | 3 | 0.8557 | 0.7938 | 0.8300 | 0.8200 |
| Air Quality | LSTM | mae | 7 | 0.8735 | 0.7990 | 0.8336 | 0.8196 |
| Air Quality | LSTM | rmse | 7 | 1.1638 | 1.0892 | 1.1136 | 1.1028 |
| Air Quality | LSTM | mae_95ci_low | 7 | 0.8309 | 0.7738 | 0.8096 | 0.7958 |
| Air Quality | LSTM | mae_95ci_high | 7 | 0.9161 | 0.8243 | 0.8576 | 0.8433 |
| Air Quality | LSTM | mae | 14 | 0.8742 | 0.8393 | 0.8831 | 0.8372 |
| Air Quality | LSTM | rmse | 14 | 1.1560 | 1.1304 | 1.1704 | 1.1089 |
| Air Quality | LSTM | mae_95ci_low | 14 | 0.8292 | 0.8192 | 0.8427 | 0.8030 |
| Air Quality | LSTM | mae_95ci_high | 14 | 0.9192 | 0.8595 | 0.9235 | 0.8714 |
| Air Quality | LSTM | mae | 30 | 0.9045 | 0.8298 | 0.8651 | 0.8565 |
| Air Quality | LSTM | runtime | 30 | 6.3374 | 6.7021 | 9.1254 | 26.6938 |
| Air Quality | LSTM | mae_95ci_low | 30 | 0.8668 | 0.8058 | 0.8286 | 0.8219 |
| Air Quality | LSTM | mae_95ci_high | 30 | 0.9423 | 0.8539 | 0.9017 | 0.8911 |

| | | | | | | | |
|---|---|---|---|---|---|---|---|
| Air Quality | LSTM | mae | 60 | 0.8968 | 0.8422 | 0.8824 | 0.8230 |
| Air Quality | LSTM | runtime | 60 | 22.9802 | 24.6852 | 20.3635 | 54.5859 |
| Air Quality | LSTM | mae_95ci_low | 60 | 0.8677 | 0.8131 | 0.8575 | 0.7680 |
| Air Quality | LSTM | mae_95ci_high | 60 | 0.9258 | 0.8712 | 0.9072 | 0.8780 |
| Electricity | LSTM | mae | 1 | 0.0792 | 0.0824 | 0.1038 | 0.0782 |
| Electricity | LSTM | runtime | 1 | 7.8921 | 7.8495 | 7.8987 | 95.7385 |
| Electricity | LSTM | mae_95ci_low | 1 | 0.0765 | 0.0791 | 0.1020 | 0.0755 |
| Electricity | LSTM | mae_95ci_high | 1 | 0.0818 | 0.0857 | 0.1056 | 0.0809 |
| Electricity | LSTM | mae | 3 | 0.0826 | 0.0817 | 0.1049 | 0.0800 |
| Electricity | LSTM | runtime | 3 | 7.7053 | 8.5866 | 8.8290 | 88.8553 |
| Electricity | LSTM | mae_95ci_low | 3 | 0.0773 | 0.0761 | 0.1020 | 0.0756 |
| Electricity | LSTM | mae_95ci_high | 3 | 0.0880 | 0.0873 | 0.1078 | 0.0844 |
| Electricity | LSTM | mae | 7 | 0.0812 | 0.0809 | 0.1045 | 0.0795 |
| Electricity | LSTM | runtime | 7 | 8.5592 | 9.3183 | 9.5516 | 102.5181 |
| Electricity | LSTM | mae_95ci_low | 7 | 0.0768 | 0.0791 | 0.1030 | 0.0758 |
| Electricity | LSTM | mae_95ci_high | 7 | 0.0856 | 0.0826 | 0.1059 | 0.0832 |
| Electricity | LSTM | mae | 14 | 0.0814 | 0.0832 | 0.1060 | 0.0822 |
| Electricity | LSTM | runtime | 14 | 9.3840 | 9.0948 | 9.2311 | 97.2820 |
| Electricity | LSTM | mae_95ci_low | 14 | 0.0777 | 0.0774 | 0.1045 | 0.0776 |
| Electricity | LSTM | mae_95ci_high | 14 | 0.0852 | 0.0890 | 0.1076 | 0.0867 |
| Electricity | LSTM | mae | 30 | 0.0848 | 0.0806 | 0.1056 | 0.0844 |
| Electricity | LSTM | runtime | 30 | 8.4287 | 10.1354 | 9.7164 | 99.5264 |
| Electricity | LSTM | mae_95ci_low | 30 | 0.0814 | 0.0776 | 0.1033 | 0.0804 |
| Electricity | LSTM | mae_95ci_high | 30 | 0.0883 | 0.0836 | 0.1080 | 0.0885 |
| Electricity | LSTM | mae | 60 | 0.0791 | 0.0789 | 0.1031 | 0.0802 |
| Electricity | LSTM | runtime | 60 | 9.9183 | 9.6104 | 10.2516 | 104.8715 |
| Electricity | LSTM | mae_95ci_low | 60 | 0.0770 | 0.0757 | 0.1017 | 0.0758 |
| Electricity | LSTM | mae_95ci_high | 60 | 0.0812 | 0.0822 | 0.1046 | 0.0846 |

# PatchTST Model Results

| Dataset | Model | Metric | Sequence Length | No Dropout | Dropout | MC Dropout | Synaptic Pruning |
|---|---|---|---|---|---|---|---|
| Bitcoin | PatchTST | mae | 1 | 0.1821 | 0.7143 | 0.4325 | 0.1916 |
| Bitcoin | PatchTST | runtime | 1 | 0.2219 | 0.7396 | 0.5080 | 0.2309 |
| Bitcoin | PatchTST | mae_95ci_low | 1 | 0.1418 | 0.6519 | 0.3574 | 0.1425 |
| Bitcoin | PatchTST | mae_95ci_high | 1 | 0.2225 | 0.7768 | 0.5075 | 0.2407 |
| Bitcoin | PatchTST | mae | 3 | 0.3130 | 0.6621 | 0.3317 | 0.3131 |
| Bitcoin | PatchTST | runtime | 3 | 0.3524 | 0.6877 | 0.3915 | 0.3524 |
| Bitcoin | PatchTST | mae_95ci_low | 3 | 0.1950 | 0.5242 | 0.2391 | 0.1954 |
| Bitcoin | PatchTST | mae_95ci_high | 3 | 0.4311 | 0.7999 | 0.4244 | 0.4307 |
| Bitcoin | PatchTST | mae | 7 | 0.2952 | 0.6561 | 0.3696 | 0.2810 |
| Bitcoin | PatchTST | rmse | 7 | 0.3434 | 0.6856 | 0.4277 | 0.3281 |
| Bitcoin | PatchTST | mae_95ci_low | 7 | 0.1890 | 0.5071 | 0.2686 | 0.1690 |
| Bitcoin | PatchTST | mae_95ci_high | 7 | 0.4013 | 0.8051 | 0.4705 | 0.3931 |
| Bitcoin | PatchTST | mae | 14 | 0.3173 | 0.6680 | 0.4041 | 0.3172 |
| Bitcoin | PatchTST | rmse | 14 | 0.3678 | 0.7005 | 0.4652 | 0.3677 |
| Bitcoin | PatchTST | mae_95ci_low | 14 | 0.2265 | 0.5547 | 0.3038 | 0.2263 |
| Bitcoin | PatchTST | mae_95ci_high | 14 | 0.4081 | 0.7813 | 0.5044 | 0.4082 |
| Bitcoin | PatchTST | mae | 30 | 0.4780 | 0.9609 | 0.5666 | 0.4761 |
| Bitcoin | PatchTST | rmse | 30 | 0.5245 | 0.9904 | 0.6186 | 0.5228 |
| Bitcoin | PatchTST | mae_95ci_low | 30 | 0.3573 | 0.8008 | 0.4461 | 0.3530 |
| Bitcoin | PatchTST | mae_95ci_high | 30 | 0.5987 | 1.1210 | 0.6871 | 0.5992 |
| Bitcoin | PatchTST | mae | 60 | 0.6402 | 0.9828 | 0.6674 | 0.6362 |
| Bitcoin | PatchTST | runtime | 60 | 0.6797 | 1.0121 | 0.7097 | 0.6759 |
| Bitcoin | PatchTST | mae_95ci_low | 60 | 0.5903 | 0.9323 | 0.6275 | 0.5902 |
| Bitcoin | PatchTST | mae_95ci_high | 60 | 0.6901 | 1.0334 | 0.7073 | 0.6821 |
| S&P500 | PatchTST | mae | 1 | 0.2819 | 0.4299 | 0.6804 | 0.2838 |
| S&P500 | PatchTST | rmse | 1 | 0.3408 | 0.5177 | 0.7712 | 0.3760 |
| S&P500 | PatchTST | mae_95ci_low | 1 | 0.2403 | 0.3876 | 0.6483 | 0.2711 |
| S&P500 | PatchTST | mae_95ci_high | 1 | 0.3236 | 0.4721 | 0.7124 | 0.3643 |
| S&P500 | PatchTST | mae | 3 | 0.3008 | 0.2797 | 0.5755 | 0.2925 |
| S&P500 | PatchTST | rmse | 3 | 0.3584 | 0.3624 | 0.6553 | 0.3514 |
| S&P500 | PatchTST | mae_95ci_low | 3 | 0.2641 | 0.2563 | 0.5336 | 0.2548 |
| S&P500 | PatchTST | mae_95ci_high | 3 | 0.3374 | 0.3030 | 0.6174 | 0.3301 |

| | | | | | | | |
|---|---|---|---|---|---|---|---|
| S&P500 | PatchTST | mae | 7 | 0.3180 | 0.2358 | 0.5145 | 0.2358 |
| S&P500 | PatchTST | rmse | 7 | 0.3772 | 0.3023 | 0.5892 | 0.3024 |
| S&P500 | PatchTST | mae_95ci_low | 7 | 0.2745 | 0.1998 | 0.4767 | 0.1999 |
| S&P500 | PatchTST | mae_95ci_high | 7 | 0.3614 | 0.2717 | 0.5523 | 0.2717 |
| S&P500 | PatchTST | mae | 14 | 0.4077 | 0.3048 | 0.5307 | 0.3121 |
| S&P500 | PatchTST | rmse | 14 | 0.4825 | 0.3918 | 0.6164 | 0.4006 |
| S&P500 | PatchTST | mae_95ci_low | 14 | 0.3675 | 0.2780 | 0.4984 | 0.2807 |
| S&P500 | PatchTST | mae_95ci_high | 14 | 0.4479 | 0.3315 | 0.5631 | 0.3436 |
| S&P500 | PatchTST | mae | 30 | 0.4779 | 0.3286 | 0.5970 | 0.3398 |
| S&P500 | PatchTST | rmse | 30 | 0.5645 | 0.4230 | 0.6886 | 0.4366 |
| S&P500 | PatchTST | mae_95ci_low | 30 | 0.4470 | 0.2957 | 0.5514 | 0.3145 |
| S&P500 | PatchTST | mae_95ci_high | 30 | 0.5088 | 0.3616 | 0.6426 | 0.3652 |
| S&P500 | PatchTST | mae | 60 | 0.5850 | 0.4083 | 0.6555 | 0.4099 |
| S&P500 | PatchTST | rmse | 60 | 0.6708 | 0.5186 | 0.7415 | 0.5208 |
| S&P500 | PatchTST | mae_95ci_low | 60 | 0.5320 | 0.3573 | 0.6054 | 0.3602 |
| S&P500 | PatchTST | mae_95ci_high | 60 | 0.6380 | 0.4592 | 0.7056 | 0.4595 |
| Air Quality | PatchTST | mae | 1 | 16.1275 | 27.0567 | 15.9646 | 15.6985 |
| Air Quality | PatchTST | rmse | 1 | 45.3082 | 53.2031 | 45.4585 | 45.0086 |
| Air Quality | PatchTST | mae_95ci_low | 1 | 14.8850 | 25.4175 | 14.6479 | 14.1160 |
| Air Quality | PatchTST | mae_95ci_high | 1 | 17.3700 | 28.6960 | 17.2813 | 17.2810 |
| Air Quality | PatchTST | mae | 3 | 19.7196 | 22.5570 | 15.2132 | 19.9416 |
| Air Quality | PatchTST | rmse | 3 | 43.8000 | 46.8524 | 42.7943 | 43.8994 |
| Air Quality | PatchTST | mae_95ci_low | 3 | 13.0623 | 17.3900 | 13.7394 | 12.9484 |
| Air Quality | PatchTST | mae_95ci_high | 3 | 26.3769 | 27.7240 | 16.6871 | 26.9347 |
| Air Quality | PatchTST | mae | 7 | 16.2646 | 20.0300 | 15.6466 | 15.9935 |
| Air Quality | PatchTST | rmse | 7 | 43.0241 | 45.9279 | 42.7583 | 43.0292 |
| Air Quality | PatchTST | mae_95ci_low | 7 | 11.5829 | 14.2740 | 12.0707 | 12.4944 |
| Air Quality | PatchTST | mae_95ci_high | 7 | 20.9463 | 25.7861 | 19.2225 | 19.4926 |
| Air Quality | PatchTST | mae | 14 | 19.3945 | 21.5496 | 17.5457 | 18.3663 |
| Air Quality | PatchTST | rmse | 14 | 43.3334 | 46.6010 | 43.2483 | 43.7783 |
| Air Quality | PatchTST | mae_95ci_low | 14 | 15.3269 | 15.5848 | 13.4590 | 14.2256 |
| Air Quality | PatchTST | mae_95ci_high | 14 | 23.4622 | 27.5145 | 21.6323 | 22.5071 |
| Air Quality | PatchTST | mae | 30 | 13.7902 | 22.5991 | 16.8941 | 13.0852 |
| Air Quality | PatchTST | rmse | 30 | 44.1359 | 47.5883 | 43.8919 | 43.6895 |
| Air Quality | PatchTST | mae_95ci_low | 30 | 11.0907 | 20.0749 | 11.4158 | 11.3914 |
| Air Quality | PatchTST | mae_95ci_high | 30 | 16.4896 | 25.1234 | 22.3725 | 14.7790 |

| | | | | | | | |
|---|---|---|---|---|---|---|---|
| Air Quality | PatchTST | mae | 60 | 20.8918 | 27.2025 | 17.7279 | 18.1252 |
| Air Quality | PatchTST | rmse | 60 | 50.0566 | 54.5919 | 46.9463 | 47.3044 |
| Air Quality | PatchTST | mae_95ci_low | 60 | 10.7801 | 21.5402 | 15.0372 | 13.6740 |
| Air Quality | PatchTST | mae_95ci_high | 60 | 31.0035 | 32.8647 | 20.4186 | 22.5763 |
| Electricity | PatchTST | mae | 1 | 0.1009 | 0.2832 | 0.1447 | 0.0989 |
| Electricity | PatchTST | rmse | 1 | 0.1859 | 0.3637 | 0.2240 | 0.1857 |
| Electricity | PatchTST | mae_95ci_low | 1 | 0.0902 | 0.2655 | 0.1408 | 0.0862 |
| Electricity | PatchTST | mae_95ci_high | 1 | 0.1117 | 0.3009 | 0.1487 | 0.1116 |
| Electricity | PatchTST | mae | 3 | 0.1146 | 0.3411 | 0.1331 | 0.1070 |
| Electricity | PatchTST | rmse | 3 | 0.1909 | 0.4212 | 0.2121 | 0.1862 |
| Electricity | PatchTST | mae_95ci_low | 3 | 0.0990 | 0.3022 | 0.1248 | 0.0916 |
| Electricity | PatchTST | mae_95ci_high | 3 | 0.1302 | 0.3800 | 0.1414 | 0.1223 |
| Electricity | PatchTST | mae | 7 | 0.1015 | 0.3279 | 0.1265 | 0.1014 |
| Electricity | PatchTST | rmse | 7 | 0.1822 | 0.4084 | 0.2038 | 0.1825 |
| Electricity | PatchTST | mae_95ci_low | 7 | 0.0893 | 0.2902 | 0.1149 | 0.0894 |
| Electricity | PatchTST | mae_95ci_high | 7 | 0.1137 | 0.3657 | 0.1381 | 0.1134 |
| Electricity | PatchTST | mae | 14 | 0.1011 | 0.3079 | 0.1310 | 0.0952 |
| Electricity | PatchTST | rmse | 14 | 0.1847 | 0.3856 | 0.2071 | 0.1825 |
| Electricity | PatchTST | mae_95ci_low | 14 | 0.0867 | 0.2902 | 0.1160 | 0.0819 |
| Electricity | PatchTST | mae_95ci_high | 14 | 0.1154 | 0.3256 | 0.1460 | 0.1084 |
| Electricity | PatchTST | mae | 30 | 0.1214 | 0.2879 | 0.1233 | 0.1175 |
| Electricity | PatchTST | rmse | 30 | 0.1976 | 0.3653 | 0.1993 | 0.1957 |
| Electricity | PatchTST | mae_95ci_low | 30 | 0.1003 | 0.2594 | 0.1149 | 0.0967 |
| Electricity | PatchTST | mae_95ci_high | 30 | 0.1425 | 0.3165 | 0.1317 | 0.1383 |
| Electricity | PatchTST | mae | 60 | 0.1218 | 0.3206 | 0.1312 | 0.1158 |
| Electricity | PatchTST | rmse | 60 | 0.2049 | 0.3934 | 0.2076 | 0.2018 |
| Electricity | PatchTST | mae_95ci_low | 60 | 0.1057 | 0.2765 | 0.1185 | 0.0990 |
| Electricity | PatchTST | mae_95ci_high | 60 | 0.1379 | 0.3646 | 0.1440 | 0.1325 |
